# Supplementary material for: Photon-mediated interactions between quantum emitters in a diamond nanocavity
Source: arXiv:1807.04265 ancillary file (2018-07-11)
Supplement: Supplementary file 1 [file Two_SiV_Interactions_SI.pdf]

# Supplementary Material for: Photon-mediated interactions between quantum emitters in a diamond nanocavity

R. E. Evans[1,*], M. K. Bhaskar[1,*], D. D. Sukachev[1,*], C. T. Nguyen[1],
A. Sipahigil[1], M. J. Burek[2], B. Machielse[1,2], G. H. Zhang[1],
A. S. Zibrov[1], E. Bielejec[3], H. Park[1,4], M. Lončar[2], M. D. Lukin[1,†]
[1]Department of Physics, Harvard University, Cambridge, MA 02138, USA
[2]John A. Paulson School of Engineering and Applied Sciences,
Harvard University, Cambridge, MA 02138, USA
[3]Sandia National Laboratories, Albuquerque, NM 87185, USA
[4]Department of Chemistry and Chemical Biology,
Harvard University, Cambridge, MA 02138, USA
[*] These authors contributed equally to this work.
[†] Corresponding author. E-mail: lukin@physics.harvard.edu

July 10, 2018

# Materials and Methods

## Contents


**1 Experimental setup** **3**
- 1.1 Confocal microscopy inside a dilution refrigerator . . . . . . . . . . . . . . . . . . 3
- 1.2 Excitation and readout of the diamond nanodevice . . . . . . . . . . . . . . . . . . 5
- 1.3 Fiber-based photon collection and polarization control . . . . . . . . . . . . . . 5
- 1.4 Gas tuning of the nanocavity resonance . . . . . . . . . . . . . . . . . . . . . . . . . 7

**2 Model for two SiV centers inside an optical cavity** **8**

**3 Single-SiV measurements** **10**
- 3.1 Verification of single SiV centers . . . . . . . . . . . . . . . . . . . . . . . . . . . . 10
- 3.2 Extraction of cavity QED parameters . . . . . . . . . . . . . . . . . . . . . . . . . . 11
- 3.3 Additional factors influencing the cavity transmission spectrum . . . . . . . . . 12

**4 Two-SiV transmission measurements in zero magnetic field** **13**
- 4.1 Charge-state control of SiV centers . . . . . . . . . . . . . . . . . . . . . . . . . . . 13
- 4.2 Spectral hopping of SiV centers . . . . . . . . . . . . . . . . . . . . . . . . . . . . . 13
- 4.3 Bright and dark state linewidth measurements . . . . . . . . . . . . . . . . . . . . 14
- 4.4 Cavity QED parameters for the two-SiV measurements in zero magnetic field . 14

**5 Fidelity calculation for single-shot readout of the SiV spin** **16**

**6 Spin-dependent SiV-cavity transmission on cavity resonance** **17**

**7 Two-SiV transmission measurements in nonzero magnetic fields** **18**
- 7.1 SiV frequency stabilization based on active preselection . . . . . . . . . . . . . 18
- 7.2 Zeeman splitting calibration . . . . . . . . . . . . . . . . . . . . . . . . . . . . . . . 19
- 7.3 Spin-dependent measurement of the two-SiV transmission spectra . . . . . . . 19
- 7.4 Cavity QED parameters for the two-SiV measurements in a non-zero magnetic field . . . . . . . . . . . . . . . . . . . . . . . . . . . . . . . . . . . . . . . . . . . . . 20
- 7.5 Measurement of collective-state formation in an independent device . . . . . . 21

# 1 Experimental setup

## 1.1 Confocal microscopy inside a dilution refrigerator

All experiments are carried out in a dilution refrigerator (DR: BlueFors BF-LD250) with free-space optical access (see **Fig. S1**). To perform scanning confocal microscopy, we use a dual-axis scanning galvonometer mirror system (Thorlabs GVS012), two concatenated $4f$ lens systems ($f_1 = f_3 = 25\,\mathrm{cm}$, $f_2 = 30\,\mathrm{cm}$, $f_4 = 20\,\mathrm{cm}$) consisting of anti-reflection coated, $40\,\mathrm{mm}$-diameter cemented achromatic doublets (VIS-NIR, Edumund Optics) and a vacuum- and cryo-compatible objective (Attocube LT-APO-VISIR, NA = 0.82) to deliver light to the diamond nanodevice. Light reflected from the sample through the microscope is partially reflected by a 33:67 pellicle beam splitter to a CCD camera for imaging.

A 6-1-1 T superconducting vector magnet (American Magnetics Inc.) is mounted below the mixing chamber (MXC) and thermally linked to the 4 K plate of the DR. The magnet is operated in persistent current mode to maximize the stability of the applied field used for Zeeman splitting of the SiV spin states. The diamond substrate containing the nanodevices is soldered with indium to a copper sample stage and placed inside the magnet bore. A temperature sensor (Lake Shore Cryotronics, RX-102B-CB) is attached to the sample holder and measures a base temperature of $85\,\mathrm{mK}$.

The objective lens is mounted on a piezoelectric stepper (Attocube ANPx311) via an L-bracket. We use the stepper to move the objective to adjust the focus. The sample stage sits directly beneath the objective, next to an aluminum mount which holds the tapered tip of the optical fiber, through which light exits (and, in some experiments, enters) the DR. The fiber holder is mounted on a stack of 3-axis piezoelectric steppers ($2\times$ Attocube ANPx101, $1\times$ Attocube ANPz101). These steppers are used to position the fiber relative to the nanodevice, allowing us to maximize the coupling efficiency to the tapered diamond waveguide and couple to multiple devices without bringing the DR above $4\,\mathrm{K}$ or exchanging the sample. The sample stage and fiber mount stepper stack are both on the copper science plate, which is attached to a separate stack of $x$- and $y$-axis piezoelectric steppers ($2\times$ Attocube ANPx311) on top of the base plate. These steppers are used for simultaneous positioning of both the sample stage and the fiber mount relative to the microscope objective.

The base plate is connected to the MXC via thick copper beams which provide a thermal connection as well as a rigid mechanical link, minimizing vibrations propagating mostly from the pulse tube and hence reducing the pointing error of the confocal microscope to approximately $1\,\mu\mathrm{m}$ in amplitude. The sample stage, objective L-bracket and aluminum thermalization plates (inserted between neighboring base steppers) are also thermally anchored to the MXC via connection to the base plate by oxygen-free copper braids (Copper Braid Products, not shown in **Fig. S1**). This ensures rapid thermalization of the entire sample stage setup and inhibits slow mechanical drift of the fiber and objective during the experiment.

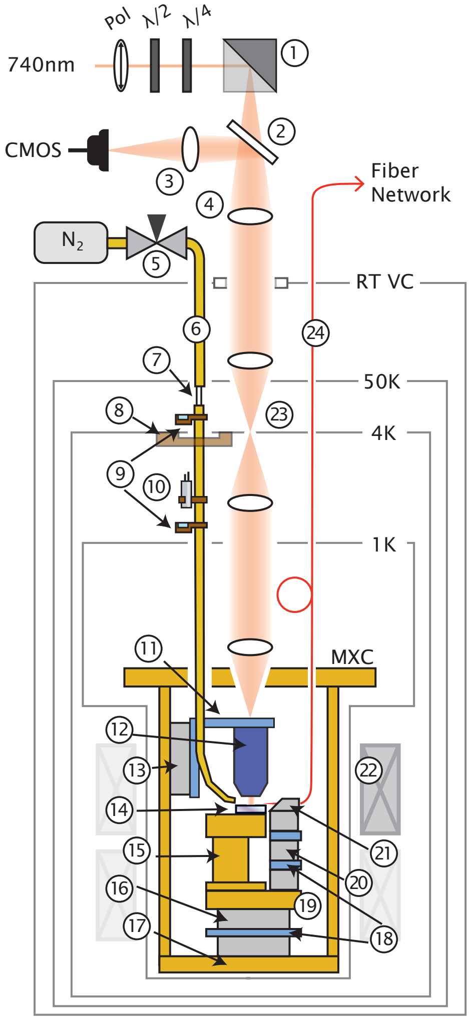


Figure S1: Schematic of the confocal microscope inside a dilution refrigerator (DR). RT VC: Outer vacuum can at room temperature; 50K: $50\,\mathrm{K}$ plate; 4K: $4\,\mathrm{K}$ plate; 1K: $1\,\mathrm{K}$ plate; MXC: Mixing chamber plate; CMOS: CMOS camera; Pol, $\lambda/2$, $\lambda/4$: Polarizer, half-wave plate, quarter-wave plate; 1: dual-axis scanning galvonometer mirror system (Thorlabs GVS012); 2: 33:67 pellicle beam splitter; 3: achromatic lens ($f = 10\,\mathrm{cm}$); 4: $40\,\mathrm{mm}$ diameter achromatic lenses ($f_1 = f_3 = 25\,\mathrm{cm}$, $f_2 = 30\,\mathrm{cm}$, $f_4 = 20\,\mathrm{cm}$); 5: tunable leak valve (VAT Series 211 DN 16 No. 21124-KE0X-000); 6: Copper tube which delivers the $N_2$ for gas tuning (see sec. 1.4); 7: PTFE thermal break; 8: copper thermal link; 9: temperature sensors (Lake Shore DT-670); 10: resistive cartridge heater (Lake Shore HTR-50); 11: objective L-bracket; 12: vacuum- and cryo-compatible objective (Attocube LT-APO-VISIR, NA = 0.82, focal length = $2.87\,\mathrm{mm}$); 13: piezoelectric stepper (Attocube ANPx311) which adjusts the focus of the objective; 14: diamond substrate containing nanodevice; 15: sample stage; 16: piezoelectric steppers (Attocube ANPx311) which position the stage and fiber mount laterally; 17: base plate; 18: aluminum thermalization plates; 19: science plate; 20: piezoelectric steppers (Attocube: $2\times$ ANPx101, $1\times$ ANPz101) which position the fiber mount; 21: fiber mount; 22: 6-1-1 T superconducting vector magnet with persistent switches (American Magnetics Inc. MAxes); 23: $10\,\mathrm{mm}$ aperture at 4 K plate of the DR; 24: single-mode fiber (S630-HP). All parts shown in brown or gold are copper (C101). All parts shown in light blue are aluminum (Al 6061).

## 1.2 Excitation and readout of the diamond nanodevice

A full description of the diamond nanodevice and its fabrication procedure are presented elsewhere (*25*). The nanodevice consists of a 1D photonic crystal cavity symmetrically coupled to a waveguide. The waveguide has two ports. The first port is a notch that couples free-space light entering from the confocal microscope into the waveguide. Light entering through this path is used for resonant excitation of the SiV and cavity modes and comes from narrow-band lasers [Newport TLB-6711, M-Squared SolsTiS-2000-PSX-XF and a home-built external-cavity diode laser (Opnext Diode HL7302MG, Littrow configuration)]. In some experiments (see Sec. 7.1), these lasers are modulated using an electro-optic phase modulator (EOSPACE model PM-0S5-10-PFA-PFA-740-SUL) with microwave sources (MW: Agilent 83732B and Hittite HMC-T2220) to generate additional optical frequencies. The second port is the tapered end of the nanobeam waveguide, which is contacted to the tapered tip of a single mode optical fiber. The coupled fiber is then used to collect light from the cavity mode propagating out of the waveguide. Our techniques for chemically fabricating the tapered fiber and performing the coupling are described in previous works (*21, 25*). We also apply pulses from a $520\,\mathrm{nm}$ diode laser (Thorlabs LP520-SF15) via the tapered fiber, as shown in **Fig. S2**, for charge-state control of the SiV (described in detail in Sec. 7.1).

## 1.3 Fiber-based photon collection and polarization control

A fiber-based optical network (**Fig. S2**) is used to efficiently collect light transmitted through the waveguide. In this section, we discuss the use of this fiber network to measure the coupling efficiency of the tapered optical fiber to the diamond waveguide, to control the polarization of the input and output light in the fiber, and to measure the broadband response of the diamond nanocavity.

To couple the tapered fiber to the waveguide, we first send light from a supercontinuum light source (NKT Photonics SuperKExtreme) into the fiber network. The input light is spectrally filtered to an approximately $10\,\mathrm{nm}$ range around the SiV ZPL wavelength (Semrock FF01-740/13-25) and then sent into a 90:10 fiber beamsplitter, with $90\%$ of the light sent to a calibration photodiode, and the remaining $10\%$ sent into the diamond waveguide through the tapered fiber contact. The light reflected from the cavity is then split by two other 90:10 beam splitters, which send $1\%$ of the final output light to a reflection photodiode. The efficiency of the coupling between the fiber and the tapered end of the waveguide is calculated by comparing the incoming power and the reflected power measured from the two photodiodes. For this experiment, the frequency of the light is within the stopband of the photonic crystal cavity, and the polarization of the light is adjusted so that it couples only to the correct mode of the device (see below). Therefore, the light should be perfectly reflected. Imperfections in either of these areas will cause us to underestimate the coupling efficiency. For the experiments in this paper, we

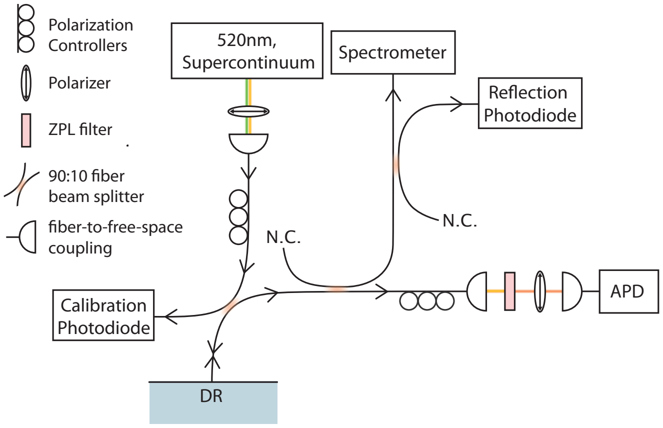


Figure S2: Schematic of the fiber network used for efficient collection of light from the diamond waveguide. The polarization of the input and output light of the diamond nanocavity inside the DR is tuned via separate sets of polarizers and polarization controllers. The fiber-waveguide coupling efficiency is measured by splitting the light entering and exiting the DR to a calibration photodiode and a reflection photodiode, respectively, and comparing the two signals. The collected light is filtered through a narrowband filter (Semrock FF01-740/13-25) centered around the SiV ZPL wavelength before being detected. N.C. indicates no connection.

infer a fiber-waveguide coupling efficiency of approximately $50\%$.

We measure a transmission efficiency of approximately $10\%$ along the fiber collection path, which accounts for losses from beam splitters, four fiber splices with an average efficiency of $80\%$ per splice and the free-space frequency-filtering stage. With the fiber-waveguide coupling efficiency of around $50\%$ described above and an SPCM efficiency of around $50\%$, the total detection efficiency of light from the diamond nanocavity is approximately $2.5\%$.

The waveguide supports two polarization modes: a transverse-electric-like (TE) mode corresponding to the cavity polarization and an orthogonal transverse-magnetic-like (TM) mode with no spectrally-similar cavity resonance. We tune the polarizations of both the input and output fields to address the TE mode of the device. The input resonant-excitation light beam consists of light from different narrowband lasers joined via fiber-based beamsplitters, and couples from free space into the waveguide. We control the polarization of this input field using a polarizer, half wave-plate, and a quarter wave-plate placed in the beam path as shown in **Fig. S1**.

Polarization control of the output light transmitted through the diamond waveguide is achieved using the fiber network: First, light propagating out from the diamond waveguide couples to the tapered optical fiber which exits the DR. The light then passes through a polarizer and a set of polarization controllers before being filtered to a frequency range around the ZPL via a band-pass filter (Semrock FF01-740/13-25) in free-space and coupled back into a fiber and collected

by a single-photon counting module ("SPCM"; Excelitas SPCM-NIR). By tuning the polarizer and polarization controllers while monitoring the photon detection rate, we can minimize the detection rate at a frequency far detuned from the cavity resonance, where a non-zero spectrally-flat background signal indicates transmission of the TM mode. As a result, the relative signal from the cavity (TE) mode of interest is maximized.

We can also use the fiber network to perform characterization of the spectrum of the diamond nanocavity via reflection. For low-resolution characterization of the diamond nanocavity, light from the broadband supercontinuum laser (with no spectral filtering) is sent in from the fiber for non-resonant excitation of the system. A separate polarizer and set of polarization controllers tune the polarization of this input light to selectively address the nanocavity mode. Reflected light from the cavity is coupled back into the tapered fiber and collected through the fiber and sent to a spectrometer (Horiba iHR550 with Synapse CCD and $1800\,\mathrm{gr/mm}$) with a spectral resolution of $0.025\,\mathrm{nm}$.

## 1.4 Gas tuning of the nanocavity resonance

We tune the resonance wavelength of the diamond nanocavity by depositing solid $N_2$ on the diamond waveguide to change its refractive index. As shown in **Fig. S1**, $N_2$ gas is extracted from a reservoir at atmospheric pressure via a tunable leak valve (VAT Series 211 DN 16 No. 21124-KE0X-000) into a copper tube. A vacuum gauge attached to the top of the tube is used to read out the pressure of the gas inside the tube. The tube extends into the DR and terminates at the sample stage, where $N_2$ exits and deposits onto the diamond nanocavity. To start the $N_2$ deposition, the temperature of the tube is increased by applying power of around $10\,\mathrm{W}$ to a heater resistor, attached to the tube directly below the $4\,\mathrm{K}$ stage, and monitored by several temperature sensors (Lake Shore DT-670SD) placed along the tube. As the temperature of the tube increases, the pressure inside the tube, monitored on the vacuum gauge, initially rises. When the tube reaches a temperature of roughly 80-$100\,\mathrm{K}$ near the $4\,\mathrm{K}$ plate, the pressure reaches a maximum and then starts to decrease. At this time, residual frozen $N_2$ has unclogged inside the tube and begins to flow out and deposit onto the nanodevice. We then open the leak valve to let more $N_2$ into the tube while monitoring the cavity spectrum, and close the leak valve once we have observed a satisfactory shift in the cavity resonance wavelength. The leak rate is on the order of $10^{-2}$ mbar L/s, corresponding to a cavity resonance tuning rate of approximately 0.01 nm/s. The leak rate can be adjusted in real time to control the tuning rate. The heater is then switched off and the system equilibrates.

Crucially, the copper tube has a weak but non-negligible thermal link to the $4\,\mathrm{K}$ plate, while being thermally isolated from the room-temperature environment via a PTFE thermal break below the $50\,\mathrm{K}$ plate (see **Fig. S1**). The copper tube is also carefully thermally isolated from the components of the experiment that are below $4\,\mathrm{K}$. Therefore, when the heater is off, the tube equilibriates to around $4\,\mathrm{K}$. Since this is well below the $N_2$ freezing point, $N_2$ cannot leak out

of the tube. Thus, after gas tuning, the cavity resonance wavelength experiences no drift and has been measured to be stable (to within $5\,\mathrm{GHz}$ or better) over several weeks.

While deposition of $N_2$ on the device increases the resonance wavelength, the amount of $N_2$ can also be reduced to incrementally decrease the resonance wavelength. This is done using the supercontinuum laser, which is typically used for low-resolution cavity spectra measurements through the tapered fiber connected to the diamond waveguide as described in Sec. 1.3. By applying this laser at higher power, we heat up the nanobeam and thus evaporate the deposited $N_2$. We can therefore tune the resonance wavelength of the cavity in both directions while simultaneously monitoring the cavity spectrum on the spectrometer.

# 2 Model for two SiV centers inside an optical cavity

To theoretically describe the transmission measurements described in Figures 1, 2, and 4 of the main text, we model the steady-state response of the SiV-cavity system in the linear regime using a non-Hermitian effective Hamiltonian. This approach accounts for photon loss through the cavity (decay rate $\kappa$) and through spontaneous emission ($\gamma_i$ for SiV $i$). Because there is no distinction in this formalism between photon loss and pure dephasing of the optical excited state, the $\gamma_i$ include all sources of decay and decoherence for these states.[1] Recalling the Tavis-Cummings Hamiltonian for the N-emitter case,

$$H_{\mathrm{TC,N}}/\hbar = \omega_c \hat{a}^\dagger \hat{a} + \sum_i^N \omega_i \hat{\sigma}_i^\dagger \hat{\sigma}_i + \sum_i^N g_i \left( \hat{a}^\dagger \hat{\sigma}_i + \hat{\sigma}_i^\dagger \hat{a} \right) \tag{1}$$

we write a non-Hermitian two-emitter Tavis-Cummings Hamiltonian (*42*):

$$\hat{H}_{\mathrm{TC}} = (\omega_c + \Delta - \frac{\delta}{2} - i\gamma_1)\hat{\sigma}_1^\dagger \hat{\sigma}_1 + (\omega_c + \Delta + \frac{\delta}{2} - i\gamma_2)\hat{\sigma}_2^\dagger \hat{\sigma}_2 + (\omega_c - i\kappa)\hat{a}^\dagger \hat{a} + \left[ \hat{a}^\dagger \left( g_1 \hat{\sigma}_1 + g_2 \hat{\sigma}_2 \right) + h.c. \right] \tag{2}$$

where $\omega_c$ is the frequency of the cavity, $\Delta$ is the detuning between the center-of-mass frequency of the two SiVs $(\omega_1 + \omega_2)/2$ and the cavity mode, $\delta = \omega_1 - \omega_2$ is the detuning between the two SiVs and $g_j$ is the single-photon Rabi frequency for SiV $j \in \{1, 2\}$. The operators $\hat{a}$ and $\hat{\sigma}_j$ are the annihilation operators for the cavity and SiV $j$ excitations. The spectrum of this Hamiltonian gives the bright and dark state energies *e.g.* the red and blue lines in **Fig. 4D/E**.

To calculate the transmission of the system, we use the input-output formalism (*43*) to solve for the dynamics of the cavity field $\hat{a}$:

$$\dot{\hat{a}}(t) = -i \left[ \hat{H}_{\mathrm{TC}}, \hat{a}(t) \right] + \sqrt{\kappa_{\mathrm{a}}} \hat{a}_{in}(t) + \sqrt{\kappa_{\mathrm{b}}} \hat{b}_{in}(t) - \frac{1}{2}(\kappa_{\mathrm{a}} + \kappa_{\mathrm{b}}) \hat{a}(t), \tag{3}$$

[1]Note that for consistency with the literature, we have taken $\gamma_i$ to be the *energy* decay rate, which therefore enters with a factor of $\frac{1}{2}$ in the non-Hermitian Hamiltonian (Eqn. 2) for the field amplitudes. However, this means that pure dephasing at a rate $\gamma_d$ should be included as $\gamma_i \to \gamma_i + 2\gamma_d$.

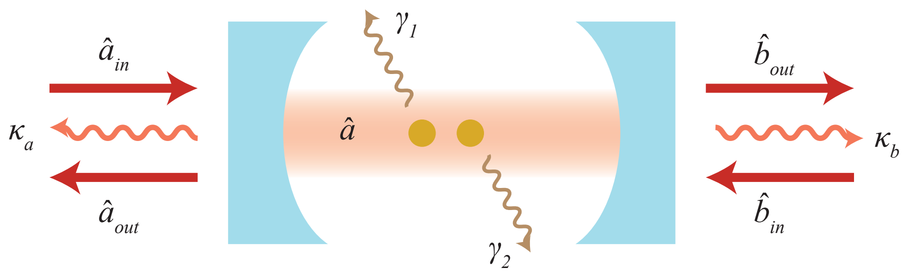


Figure S3: Visual representation of the cavity input fields $\hat{a}_{in}$ and $\hat{b}_{in} = 0$, cavity output fields $\hat{b}_{out}$ and $\hat{a}_{out}$, intra-cavity field $\hat{a}$, cavity decay $\kappa_a$ and $\kappa_b$ and SiV $i$ decoherence (including decay) $\gamma_i$.

Here, we have defined $\hat{a}_{\text{in}}$ and $\hat{b}_{\text{in}}$ as the input fields on either side of the cavity with $\kappa_{\text{a}}$ and $\kappa_{\text{b}}$ as the corresponding cavity energy decay rates and thus the total decay rate $\kappa = \kappa_{\text{a}} + \kappa_{\text{b}}$. See **Fig. S3**. (In Eqn. 3, we do not include the cavity decay term $i\kappa\hat{a}^\dagger\hat{a}$ in $H_{\text{TC}}$ since this term is already included via $\kappa_{a,b}$.) We write down the equations of motion in the frequency domain, using

$$\hat{a}(t) = \int d\omega e^{-i\omega t}\hat{a}(\omega) \tag{4}$$

to arrive at:

$$\begin{aligned} -i\omega\hat{a}(\omega) &= \left(-i\omega_c - \frac{\kappa_{\text{a}} + \kappa_{\text{b}}}{2}\right)\hat{a} + \sqrt{\kappa_{\text{a}}}\hat{a}_{\text{in}} + \sqrt{\kappa_{\text{b}}}\hat{b}_{\text{in}} - ig_1\sigma_1 - ig_2\sigma_2 \\ -i\omega\hat{\sigma}_j(\omega) &= \left(-i\left(\omega_c + \Delta + (-1)^j\frac{\delta}{2}\right) - \frac{\gamma_j}{2}\right)\hat{\sigma}_j - ig_j^*\hat{a} \end{aligned} \tag{5}$$

Eliminating the SiV degrees of freedom and solving for the cavity mode gives:

$$\hat{a}(\omega) = \frac{\sqrt{\kappa_{\text{a}}}\hat{a}_{in}(\omega) + \sqrt{\kappa_{\text{b}}}\hat{b}_{in}(\omega)}{D}, \tag{6}$$

where we have defined

$$D \equiv i(\omega_c - \omega) + \frac{\kappa_{\text{a}} + \kappa_{\text{b}}}{2} - \left(\frac{|g_1|^2}{-i\left(\omega_c - \omega + \Delta - \frac{\delta}{2}\right) - \frac{\gamma_1}{2}} + \frac{|g_2|^2}{-i\left(\omega_c - \omega + \Delta + \frac{\delta}{2}\right) - \frac{\gamma_2}{2}}\right). \tag{7}$$

In our case of interest, $\langle\hat{b}_{\text{in}}\rangle = 0$, and the transmission coefficient is $t = \langle\hat{b}_{\text{out}}\rangle/\langle\hat{a}_{\text{in}}\rangle$. Using the input-output relations $\hat{a}_{\text{out}} + \hat{a}_{\text{in}} = \sqrt{\kappa_{\text{a}}}\hat{a}$ and $\hat{b}_{\text{out}} + \hat{b}_{\text{in}} = \hat{b}_{\text{out}} = \sqrt{\kappa_{\text{b}}}\hat{a}$, we have

$$t(\omega) = \frac{\sqrt{\kappa_{\text{b}}\kappa_{\text{a}}}}{D}, \tag{8}$$

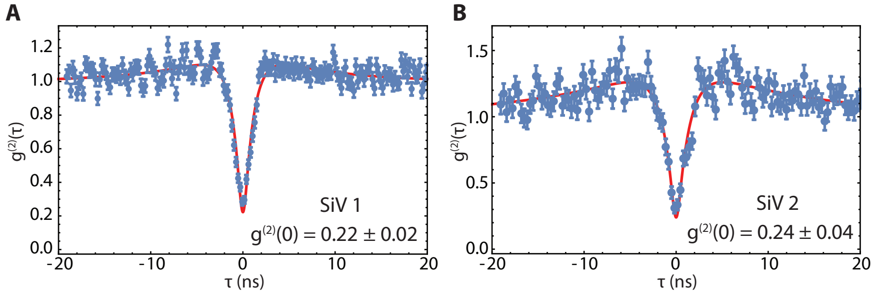


Figure S4: **Verification of single emitters.** Photon autocorrelation function $g^{(2)}(\tau)$ for SiV 1 **(A)** and SiV 2 **(B)** in the main text. Error bars are given by shot noise, and red solid lines are a fit to a model given by a double-exponential convolved with a Gaussian of $350\,\mathrm{ps}$ width to account for finite APD timing resolution. From the fits, we extract timescales for antibunching and bunching $\{\tau_{a1}, \tau_{a2}, \tau_{b1}, \tau_{b2}\} = \{1.0, 1.3, 7.7, 13.4\}$ ns.

and thus the transmission intensity for the cavity field $T(\omega) = |t(\omega)|^2$ is,

$$T(\omega) = \frac{\kappa_\mathrm{a}\kappa_\mathrm{b}}{|D|^2} \tag{9}$$

This transmission response is accurate in both the resonant and detuned regime and agrees with numerical solutions of the master equation to better than a few percent. However, to more accurately model the spectra measured in the experiment, we additionally include a background term corresponding to the leakage of coherent laser light into our detection path, resulting in a measured transmission intensity of

$$T(\omega) = |t(\omega) + Ae^{i\phi}|^2 \tag{10}$$

where $A$ and $\phi$ are the amplitude and phase of the of the background field. This coherent background term, which has a flat frequency spectrum corresponding to, for example, transmission of the TM cavity mode which is imperfectly filtered out, is necessary to account for the lineshapes we observe, which do not agree perfectly with the prediction from Eqn. 9. Addition of an incoherent background term does not appreciatively improve the agreement between the model and experiment. The solid curves in **Figs. 1, 2** and **4** in the main text are all generated via this model.

# 3 Single-SiV measurements

## 3.1 Verification of single SiV centers

In order to verify that the two emitters used in the measurements described in the main text are indeed single emitters, we separately measure the second-order correlation function $g^{(2)}(\tau)$ of

the light transmitted via each of the two SiV-like dressed states (polaritons) in the dispersive regime ($\Delta > \kappa$). Here, $\tau$ is the delay time between detection of the second and first photon. We measure under conditions where the two SiVs are far detuned from one another ($\delta \sim 2\pi\times$ 5 GHz), allowing us to measure one SiV at a time with negligible effects from their interaction. In this regime, each single SiV is only slightly dressed by the cavity mode, and acts as a transmission channel for single photons far detuned from cavity resonance. Therefore, in the ideal case, we expect $g^{(2)}(\tau = 0) \approx 0$ in transmission for single SiV-like polaritons. As explained below, a background field or limited cooperativity can increase the measured value of $g^{(2)}(0)$, but a value of $g^{(2)}(0) < 0.5$ confirms that the measured field corresponds to a single-photon emitter.

We employ an active preselection sequence described in detail in Sec. 7.1 in order to ensure initialization of each SiV in the correct charge and frequency state. These measurements are done at zero magnetic field when the spin sublevels are degenerate and only a single laser is needed to continuously scatter photons from a single SiV. The SiV-like polariton is probed in transmission and the transmitted light is split on a beamsplitter and sent to two SPCMs. Photon detection times are logged using fast acquisition hardware (PicoQuant HydraHarp 400). We construct a histogram as a function of $\tau$ and normalize it to the background signal at long time delays.

We measure $g^{(2)}(0) = 0.22 \pm 0.02$ and $g^{(2)}(0) = 0.24 \pm 0.04$ in transmission on resonance with SiV 1 and SiV 2 respectively (**Fig. S4**) with an SiV-cavity center-of-mass detuning of $\Delta = 2\pi\times$ 156 GHz at a sample temperature of 5 K. No background subtraction or postselection is used. We measure bunching on a timescale significantly longer than the excited state lifetime for both SiVs, likely due to optical pumping into the metastable higher-energy orbital branch of the ground state (*21, 28*). The finite value of $g^{(2)}(0)$ primarily arises from the coherent laser background, which is minimized relative to the single-photon transmission when the SiV is excited in the linear regime (low laser power).

## 3.2 Extraction of cavity QED parameters

In this section, we describe the measurements used to extract the cavity QED parameters $(g, \kappa, \gamma)$. We extract $\kappa = 2\pi\times$ 48 GHz, the cavity decay rate, by fitting the cavity spectrum to a Lorentzian when it is detuned from the SiV resonance by more than 5 cavity linewidths (**Fig. S5A**). The measured cavity linewidth $\kappa$ can change after the gas-tuning process, where the cavity loss rate can increase due to scattering or absorption introduced by the deposited material. This effect is not perfectly reproducible and may depend on the details of the gas deposition process. As a result, $\kappa$ can vary by tens of perecent between different experiments. In order to account for this, we measure the full cavity spectrum before each experiment and use the corresponding measured cavity linewidth as $\kappa$ in the model for that particular experiment.

We extract $\gamma_1 = 2\pi\times$ 0.19 GHz, the bare (not cavity-enhanced) linewidth of the SiV, by

fitting a Lorentzian to the transmission spectrum near the resonance of SiV 1 when the cavity is detuned by $\Delta = 6.8\kappa$ (**Fig. S5C**). In this measurement, extra care was taken to reduce the laser linewidth and power in order to prevent broadening of the measured SiV linewidth from either power broadening or spectral diffusion. Although the linewidth of SiV 2 was not measured carefully in this regime, we measured nearly-identical linewidths for the two SiVs (*cf.* **Fig. 2A** or **Fig. 4B**) at a variety of detunings, suggesting that $\gamma_1 \approx \gamma_2$. We extract $g_1 \approx g_2 = 2\pi\times$ $7.3\,\mathrm{GHz}$, the single-photon Rabi frequencies for SiV 1 and SiV 2, by fitting Eqn. 10 to the measurement in the bottom panel of **Fig. 1C** of the main text with the other CQED parameters fixed.

## 3.3 Additional factors influencing the cavity transmission spectrum

In the linear regime at $\Delta = 0$ the transmission through the cavity is given by $T \approx (1+C)^{-2}$ (*cf.* Eqn. 9). For the cooperativity $C = 23$ inferred here, the expected on-resonance transmission is $T = 0.002$, corresponding to a single-SiV cavity extinction of $\Delta T/T = 99.8\%$. This is more than the roughly $95\%$ extinction demonstrated in **Fig. 1C** of the main text. This discrepancy is primarily due to imperfect polarization of the laser field. For our device (*cf.* Sec. 1.3), the TM polarization has high transmission, resulting in the addition of a coherent background that limits the transmission contrast $\Delta T/T$. This background is accounted for in Eq. 10, which fits the data in **Fig. 1C** well. Additional factors that could contribute to the background include improper charge-state initialization (blinking) and slow-timescale (non-Markovian) broadening of the line beyond $\gamma = 2\pi\times\ 0.19\,\mathrm{GHz}$ due to spectral diffusion (*21, 24*). This measurement was done at low laser power (see Sec. 4.1-4.2) to minimize these effects. The model including the coherent background term (Eqn. 10) also accurately predicts the measured spectra in the dispersive regime. For example, the solid line shown in **Fig. 1D** of the main text is a fit to

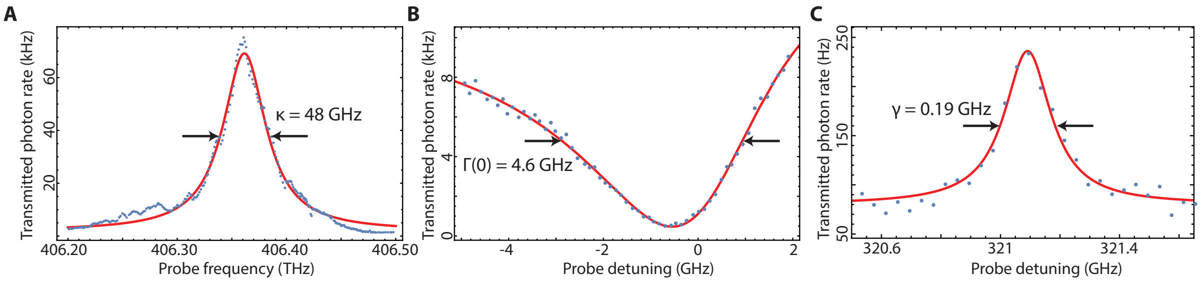


Figure S5: **Measurement of cavity and emitter linewidths (A)** Typical measurement of cavity transmission spectrum far detuned from the emitter resonance, used to extract $\kappa$. **(B)** Lorentzian with coherent background (see Sec. 2) fit to on-resonance cavity transmission near SiV 1. The data (blue points) are the same as in the lower panel of **Fig. 1C** of the main text. **(C)** Linewidth measurement of SiV 1 when the cavity is $\sim 6.8\kappa$ detuned from the SiV resonance.

Eqn. 10 with the background amplitude and phase as the only free parameters (for the exact cavity QED parameters and atom cavity detuning in this fit, see Sec. 4.4). According to this fit, the background amplitude is $12\%$ of the amplitude of the SiV-cavity signal.

We also note that since both the input and output fields are each independently filtered through a polarizer, the transmission contrast in the dispersive regime can be artificially enhanced through cross-polarization effects. While our model does not account for the two polarization modes independently, as would be necessary to completely describe the transmission signal due to this effect, our single-mode model fits the measured transmission spectra well with reasonable extracted background amplitudes.

# 4 Two-SiV transmission measurements in zero magnetic field

## 4.1 Charge-state control of SiV centers

Continuous resonant excitation of an SiV results in its eventual ionization (blinking) (*21, 24*). The ionization timescale varies among SiV centers, but at low laser powers this timescale is much longer than the time needed to measure the transmission spectrum corresponding to an SiV. This timescale can be reduced by increasing the resonant laser power, allowing us to selectively ionize a particular SiV by applying high laser power on resonance with that SiV. We can therefore ionize one of a pair of nearly-resonant SiV centers into its optically-inactive charge state and, in this way, measure the spectrum corresponding to transmission from a single SiV even when there are multiple SiV centers present (gray data in **Fig. 2A**). SiV centers can then be reinitialized with high fidelity ($\sim 80\%$) into the optically active charge state by applying a $520\,\mathrm{nm}$ laser pulse. With both SiV centers initialized in the correct charge state, we measure the two-SiV spectrum (black data in **Fig. 2A**). Because the charge state is stable over timescales longer than a single run of the experiment, we can also post-select for runs in the experiment where the two SiV centers are in the desired charge state. For more information about charge-state control of the SiV, see section 4 of the supplemental materials of Ref. (*21*).

## 4.2 Spectral hopping of SiV centers

The SiV optical transition frequency can also drift as a function of time (spectral diffusion) (*24*). While these dynamics vary from emitter to emitter, for the SiV centers studied here, we find that spectral diffusion occurs primarily in discrete spectral jumps on a timescale that increases with reduced resonant (and off-resonant repump) laser powers. For all measurements of the two-SiV system at zero magnetic field (**Fig. 2**), we work at laser intensities where the spectral diffusion timescale is much slower than the measurement timescale. In other words, we can obtain several high signal-to-noise transmission spectra before a spectral jump occurs. For example, the data

in the case of two interacting SiV centers (black curves in **Fig. 2A,B**) were each acquired over roughly $1$ minute, in which time there was no measurable spectral hopping.

SiV centers can also undergo significant spectral jumps when the sample is warmed up to room temperature and then cooled down again (thermally cycled). This means that after thermal cycling the setup, the same SiV centers can have resonance frequencies that differ on the order of $\sim 5\,\text{GHz}$. This is a much larger frequency scale than the typical slow, laser-induced spectral hopping described above ($\sim 1\,\text{GHz}$). As an example, the experiments in **Fig. 2** and **Fig. 4** of the main text were performed with the same pair of SiV centers (also labelled as SiV A and B in **Fig. 1C** of the main text). The average SiV-SiV detuning in **Fig. 2** is $\delta \sim 1\,\text{GHz}$, whereas the average SiV-SiV detuning (at zero magnetic field) in **Fig. 4** is $\delta \sim 5\,\text{GHz}$ due to this type of spectral jump. Understanding and limiting sources of spectral diffusion is an important task for future work. However, the frequency scales of all spectral hopping processes are still smaller than or comparable to the frequency tuning range of the magnetic field tuning technique demonstrated here ($\sim 5\,\text{GHz}$) and the Raman tuning technique demonstrated previously (*21*) ($\sim 20\,\text{GHz}$).

## 4.3 Bright and dark state linewidth measurements

The spectral hopping of SiV centers provides an opportunity to measure the interacting two-SiV spectra as a function of splitting between the bright and dark states by simply integrating for a long time period and binning spectra into individual sets in which no spectral hop has occured. For the measurement presented in the inset of **Fig. 2B**, we do this over the course of roughly $12$ hours and fit each binned spectrum to a double Lorentzian model (see **Fig. S6B** for some example spectra at different bright-dark splittings). To produce the plot shown in the inset of **Fig. 2B**, we bin each set of spectra based on the frequency difference between peaks obtained from the fit and plot the average width of the left (red) and right (blue) peaks in each bin. The error bars are the standard deviation within each bin. The gray dashed line and shaded region represent the mean and standard deviation of the single-SiV (that is, where the other SiV is ionized) linewidths obtained from single Lorentzian fits.

## 4.4 Cavity QED parameters for the two-SiV measurements in zero magnetic field

We determine the atom-cavity detuning $\Delta$ relative to the center-of-mass frequency of the two SiV centers using a Lorentzian fit to the spectrum shown in **Fig. S6A** ($\Delta = 2\pi\times\ 79\,\text{GHz}$) for the measurements in **Fig. 2A** and the inset of **Fig. 2B**. Using the same technique after tuning the cavity to the opposite side of the SiV resonance (for measurement in main panel of **Fig. 2B**), we estimate an SiV-cavity detuning of $\Delta = 2\pi\times\ -55\,\text{GHz}$. The cavity spectrum during these experiments ($\kappa = 2\pi\times\ 30\,\text{GHz}$) was measured to be slightly narrower than in the measurements

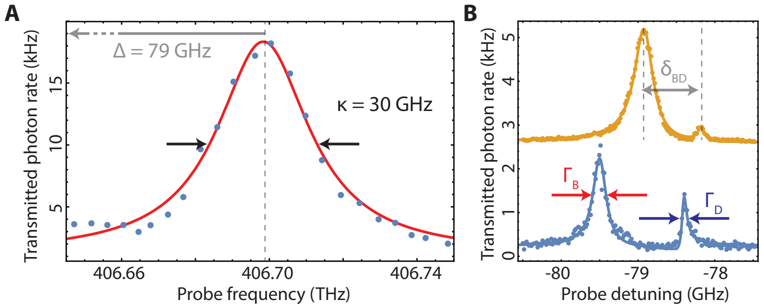


Figure S6: **Two-SiV measurement in zero magnetic field (A)** Measurement of cavity linewidth ($\kappa$) and detuning from SiV ($\Delta$) for the measurements presented in (**Fig. 1D, 2**) of the main text. The solid red line is a Lorentzian fit. **(B)** Example 2-SiV transmission spectra at different bright-dark state detunings ($\delta_{SD}$). The solid lines are a bi-Lorentzian fit with coherent background, and are used to extract $\delta_{SD}$ and the superradiant (bright) and subradiant (dark) state linewidths, $\Gamma_S$ and $\Gamma_D$, plotted in the inset of (**Fig. 3B**) in the main text.

presented in **Fig. 1** (see Sec. 3.2).

Based on these cavity spectra and the measurements described in Sec. 3, the following cavity QED parameters for the coupled SiV-cavity system are kept fixed: $\{g_1, g_2, \kappa, \gamma_1, \gamma_2\} = 2\pi \times \{7.3, 7.3, 30, 0.19, 0.19\}$ GHz yielding $C = 37$ for these SiV centers. As explained above, we set $\Delta = 2\pi\times\ 79\,\text{GHz}$ for **Fig. 2A** and the inset of **Fig. 2B** and $\Delta = 2\pi\times\ -55\,\text{GHz}$ for the main panel of **Fig. 2B**. The solid gray curves in **Fig. 2A** are single-SiV spectra obtained from Eqn. 10 by setting either $g_1$ or $g_2$ to zero. From these fits we extract the SiV-SiV detuning $\delta = 2\pi\times\ 0.56\,\text{GHz}$.

With $\Delta$ and $\delta$ fixed, we fit the two-SiV spectrum shown in black in **Fig. 2A** to Eqn. 10 with only the background terms as free parameters to obtain the solid black curve, which agrees well with the data. The close agreement between theory and experiment also validates our independently measured $g_i$ and $\gamma_i$. Since individual ionized control spectra similar to the gray data in **Fig. 2A** were not taken for the data shown in the main panel of **Fig. 2B**, $\delta$ was left as a free parameter for the fit shown in black in **Fig. 2B**, and was determined to be $\delta = 2\pi\times\ 2\,\text{GHz}$, which is different from the measured value of $\delta$ at the other cavity detuning due to the spectral diffusion process described in Sec. 4.2.

The solid lines in the inset of **Fig. 2B** are calculated with the above SiV-cavity parameters at the SiV-cavity detuning $\Delta = 2\pi\times\ 79\,\text{GHz}$, but at various $\delta$. We first calculate the energy difference between the superradiant (bright) and subradiant (dark) states as a function of SiV-SiV detuning (using the real part of the eigenvalues of $\hat{H}_{\text{TC}}$). We then calculate the $|S\rangle$ and $|D\rangle$ state linewidths (the imaginary eigenvalues of $\hat{H}_{\text{TC}}$ arising from the non-Hermitian terms) as a function of SiV-SiV detuning. This allows us to plot the theoretical bright and dark state linewidths as a function of bright and dark state energy difference, which is the parameter

determined from the fitting procedure described in Sec. 4.3 above. The solid curves in the inset of **Fig. 2** are predictions from the independently-measured cavity QED parameters (*cf.* Sec. 3.2) with no free parameters. This is because in the linear regime, the bright and dark state linewidths do not depend on the signal amplitude, laser power or background, which are the only free parameters in most of the other fits.

# 5 Fidelity calculation for single-shot readout of the SiV spin

We read out the SiV spin state in the dispersive regime by measuring the spin-dependent transmission (**Fig. 3**). The full experimental pulse sequence is shown in **Fig. S7**. The main sequence consists of a pulse at frequency $\omega_\downarrow$ which initializes the spin in $|\uparrow\rangle$ via optical pumping and a readout pulse at $\omega_\uparrow$. We build a histogram of photons in the initial time bin of duration $\delta t$, when the state is assumed to be $|\uparrow\rangle$, as well as in the final time bin of duration $\delta t$, after the system has been pumped into $|\downarrow\rangle$. These histograms represent the distribution of photon numbers we expect to observe in a single run of the experiment. Since these histograms are well separated, we can define a threshold photon number $n$ such that if the initial time bin $\delta t$ we detect more (fewer) than $n$ photons, the state is $|\uparrow\rangle$ ($|\downarrow\rangle$). We numerically optimize our choice for $\delta t$ and $n$ to maximize the single-shot readout fidelity:

$$\mathcal{F} = \text{Max}_{n,\delta t}\{(1 - \sum_{m=n}^{\infty} P_\downarrow(m,\delta t)) + (1 - \sum_{1}^{m=n} P_\uparrow(m,\delta t))\}/2. \tag{11}$$

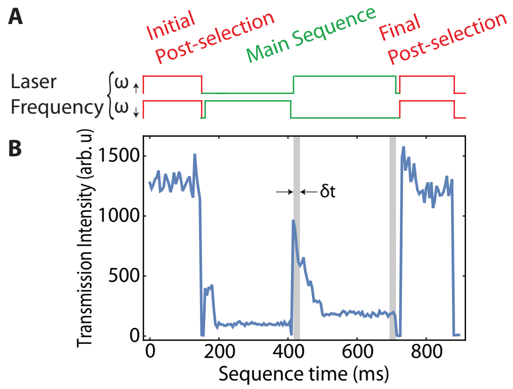


Figure S7: **Spin readout pulse sequence (A)** Pulse sequence used to measure single-shot readout and **(B)** transmission intensity as a function of time for the corresponding pulse sequence. The spin is initialized into $|\uparrow\rangle$ via optical pumping on $\omega_\downarrow$ and read out via optical pumping on $\omega_\uparrow$ (green sequences). The fidelity is calculated by comparing one time bin $\delta t$ at the beginning and end of the readout pulse (gray regions). Post-selection pulses (red) are used to ensure the experiment was initialized correctly.

To account for SiV blinking and spectral diffusion (see sec. 4), we use pre-sequence and post-sequence pulses to confirm that the SiV is at the correct frequency and in the correct charge state. Simultaneously applying two laser fields at frequencies $\omega_\uparrow$ and $\omega_\downarrow$ allows us to continuously scatter photons from the SiV without optical pumping, giving a high transmission intensity when the SiV is in the correct state. We use this pulse both at the start of the experiment (to ensure we start in the correct state) and at the end (to ensure the readout itself did not ionize the SiV).

The optimal fidelity occurs at $\delta t = 7\,\mathrm{ms}$ and $n = 34$. Without post-selection, the $|\uparrow\rangle$ histogram is bimodal, limiting the readout fidelity to $89\%$. With post-selection, the lower lobe of the histogram is removed, and the reported fidelity $\mathcal{F} = 96.8\%$ is achieved. This fidelity is not strictly the readout fidelity, but rather the combined initialization and readout fidelity. In fact, the fidelity is predominately limited by the non-zero overlap of the spin-cycling transitions used in the experiment, which can result in off-resonant pumping limiting the initialization of the spin into $|\uparrow\rangle$. Based on the measured splitting, we expect a maximum initialization and readout fidelity of $97.4\%$.

# 6 Spin-dependent SiV-cavity transmission on cavity resonance

In the main text (**Fig. 3**), we demonstrated a spin-dependent modulation of the SiV-cavity transmission response in the dispersive regime and used this effect to achieve single-shot readout of the SiV spin. We can perform a similar experiment in the resonant-cavity regime. In this regime, the SiV optical transitions are Purcell-broadened, so we apply a magnetic field of $6.5\,\mathrm{kG}$ approximately orthogonal to the SiV axis such that the splitting between the Purcell-enhanced spin transitions is maximized. We then initialize the SiV in either $|\downarrow\rangle$ or $|\uparrow\rangle$ via optical pumping (**Fig. S7A**). We probe the cavity at frequency $\omega_\uparrow$, which is resonant with both the cavity and the $|\uparrow\rangle \rightarrow |\uparrow'\rangle$ transition (**Fig. S7B**). When the spin is prepared in the state $|\downarrow\rangle$, the probe field at $\omega_\uparrow$ is detuned from the SiV transition and is transmitted (red curve). When the spin is prepared in $|\uparrow\rangle$, it couples to the probe field at frequency $\omega_\uparrow$ and the incoming light is reflected (blue curve) (*44*). We observe a maximum spin-dependent transmission contrast of 80$\%$, limited by spectral overlap between the two spin transitions. The memory time of this modulation ($50\,\mu$s) is limited by the cyclicity of the spin-conserving optical transition addressed by the probe pulse in this highly off-axis field.

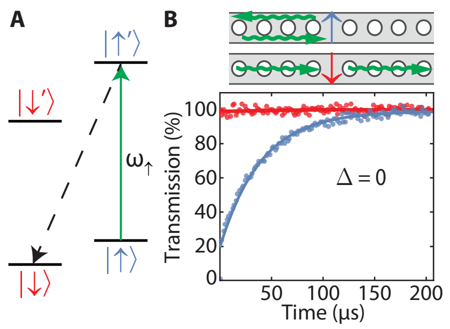


Figure S8: **Switching of the cavity transmission on resonance (A)** Simplified level structure of the SiV in a magnetic field. An optical transition at frequency $\omega_\uparrow$ (green arrow) is used to initialize the SiV spin into $|\downarrow\rangle$ by optical pumping via a spin-flipping transition (dashed line). Conversely, pumping at frequency $\omega_\downarrow$ (not shown) initializes the spin into $|\uparrow\rangle$. **(B)** Spin-dependent optical switching on cavity resonance. State $|\downarrow\rangle$ is not coupled to the probe field at frequency $\omega_\uparrow$ which is therefore transmitted (red). Initialization into $|\uparrow\rangle$ results in reflection of the probe field (blue). The maximum spin-dependent contrast is 80%.

# 7 Two-SiV transmission measurements in nonzero magnetic fields

## 7.1 SiV frequency stabilization based on active preselection

SiV optical transitions are narrow and stable for timescales long enough to enable the measurements described in **Fig. 1-3** of the main text. In order to achieve stable optical transitions over longer timescales, we use an active preselection sequence for the measurements described in **Fig. 4** of the main text. This preselection technique effectively fixes the optical transition frequencies of the emitters to desired frequencies at the expense of a slight reduction in duty cycle.

In order to cycle photons continuously from both SiV centers in a magnetic field, we apply two tones simultaneously at frequencies $\omega_{\uparrow/\downarrow,i}$ for SiV $i$ (giving four total optical frequencies). To achieve this, each SiV has one spin transition addressed by a separate resonant laser, with each laser modulated by an EOM to produce a sideband at the transition frequency of the other spin-dependent transition. For example, lasers at $\omega_{\uparrow,1}$ and $\omega_{\downarrow,2}$ have corresponding sidebands $\omega_{\downarrow,1}$ and $\omega_{\uparrow,2}$. Each SiV is separately addressed for $1\,\mathrm{ms}$ and the number of transmitted photons is recorded using a field-programmable gate array (Lattice Diamond MachXO2).

We set a photon number threshold based on observed photon count rates for these SiV centers under conditions similar to those used in the experiment. If the threshold photon number is exceeded for both SiV centers, we proceed with the experiment (typical duration: $\sim 50\,\mathrm{ms}$). If not, we apply a relatively strong ($\sim 1\,\mu\mathrm{W}$) $520\,\mathrm{nm}$ laser pulse for $100\,\mu\mathrm{s}$ to induce spectral

hopping of the SiV optical frequencies. Using this technique, we are able to measure with duty cycle $\sim 50\%$ and measure linewidths ($\sim 0.5\,\mathrm{GHz}$) that are significantly narrower than the long-timescale integrated linewidth of the SiV centers without any preselection ($\sim 2\,\mathrm{GHz}$). The gray data in **Fig. 4B** are an example of narrow lines measured using this preselection sequence.

### 7.2 Zeeman splitting calibration

We determine the frequencies of all spin-selective transitions $\omega_{\uparrow/\downarrow,i}$ as a function of magnetic field at a sample temperature of $5\,\mathrm{K}$. A complete description of the magnetic-field dependence of the SiV optical transitions can be found elsewhere (*28*). At temperatures above $500\,\mathrm{mK}$ where the relevant phonon modes are populated, working in a magnetic field misaligned with respect to the SiV symmetry axis yields a relatively short spin population relaxation rate $T_1 \sim 100\,\mathrm{ns}$ in contrast to the $50\,\mu\mathrm{s}$ for a similarly misaligned field at $85\,\mathrm{mK}$ (**Fig. 3B**) (*27*). As a result, optical pumping from a single laser at $\omega_{\uparrow/\downarrow}$ is minimal, allowing us to scatter photons at a sufficient rate to easily observe all spin transitions $\omega_{\uparrow/\downarrow,i}$ in transmission spectrum with a single laser (in other words, with no repumping laser). We measure the transmission spectra around SiV centers 1 and 2 at various magnetic fields from $0\,\mathrm{kG}$ to $8\,\mathrm{kG}$. For an example calibration transmission spectrum at $5\,\mathrm{K}$ (taken in a different device), see **Fig. S9A**.

### 7.3 Spin-dependent measurement of the two-SiV transmission spectra

For the measurements presented in **Fig. 4**, at each magnetic field value we first probe the response of SiV 1 alone by applying $\Omega_1$ continuously (to ensure initialization in $|\uparrow_1\rangle$ via optical pumping) and scanning $\Omega_p$ across the resonance. Although $\Omega_1$ is applied continuously at $\omega_{\downarrow,1}$, we only scatter photons continuously when $\Omega_p$ is on resonance with $\omega_{\uparrow,1}$ due to optical pumping into state $|\uparrow_1\rangle$ from $\Omega_1$. We then repeat the same measurement for SiV 2, applying $\Omega_2$ and scanning $\Omega_p$. One example dataset is shown in gray in **Fig. 4B**. The individual transmission spectra are then normalized to the laser background to compensate for slight differences in laser power and summed (incoherently) at each field to produce the data shown in **Fig. 4C**. At each field, we fit a Lorentzian to the single-spin spectra to determine the center frequency of the spin-selective transitions. The solid gray lines in **Fig. 4C** are linear fits to the extracted center frequencies as a function of magnetic field.

To study the two-spin interacting system, we apply $\Omega_1$ and $\Omega_2$ continuously to ensure spin initialization in $|\uparrow_1\rangle\,|\downarrow_2\rangle$ and measure the transmission spectrum of $\Omega_p$. Again, we normalize the data at each field to the background, which is primarily set by the stronger pump lasers $\Omega_1$ and $\Omega_2$. An example spectrum at a single magnetic field is shown in black in **Fig. 4B**, and the full avoided crossing (transmission spectra as a function of magnetic field) is shown in **Fig. 4D**. In all measurements (single SiV and two-SiV), we adjust our laser intensities such that $\Omega_1$ and $\Omega_2$ are roughly 3 times larger than $\Omega_p$, so that each SiV spin is polarized in the desired spin state

(spin polarization $P \sim |\Omega_{1,2}/\Omega_p|^2 \sim 90\%$).

## 7.4 Cavity QED parameters for the two-SiV measurements in a non-zero magnetic field

Despite our use of the preselection sequence described in Sec. 7.1, SiV optical transitions are broadened non-radiatively beyond the linewidth $2\pi\times$ 0.19 GHz measured on short timescales without preselection. Although this broadening has both Markovian and non-Markovian sources, to good approximation it can simply be included as an increased decoherence rate contributing to $\gamma$. Note that this approximation leads us to underestimate the SiV-cavity cooperativity.

We determine the SiV-polariton linewidth (and by extension, $\gamma$) under preselection using the single-spin transmission spectra plotted in **Fig. 4C**. By fitting Lorentzians to the individual spectra at each magnetic field (*cf.* gray data in **Fig. 4B**), we determine the mean single-SiV linewidths to be $\{\Gamma_1(\Delta), \Gamma_2(\Delta)\} = 2\pi \times \{0.77 \pm 0.14, 0.58 \pm 0.12\}$ GHz. We measure a cavity linewidth $\kappa = 2\pi\times$ 39 GHz and SiV-cavity detuning $\Delta = 2\pi\times$ 109 GHz during this measurement (not shown; see **Fig. S6A** for an example measurement) and fix $g_1 = g_2 = 2\pi\times$ 7.3 GHz as determined before. From the Purcell-enhanced linewidths and these known cavity-QED parameters, we can extract the bare SiV linewidth $\gamma$

$$\gamma_i = \Gamma_i(\Delta) - \frac{4g^2}{\kappa}\frac{1}{1 + 4\Delta^2/\kappa^2}, \tag{12}$$

yielding $\{\gamma_1, \gamma_2\} = 2\pi \times \{0.6, 0.42\}$ GHz over long timescales under preselection. We use the complete cavity QED parameters $\{g_1, g_2, \kappa, \gamma_1, \gamma_2\} = 2\pi \times \{7.3, 7.3, 39, 0.6, 0.42\}$ GHz to calculate the eigenvalues of $\hat{H}_{TC}$ at various 2-SiV detunings $\delta$ (extracted from **Fig. 4C**) which are the bright and dark state energies (solid red and blue curves in **Fig. 4D, E**). We note that these are computed using no free parameters.

In order to compare the measured data to a theoretical prediction for the full avoided-crossing transmission spectrum shown in **Fig. 4E**, we also need to include in our model effects arising from imperfect polarization $P$ into the desired spin state ($P \sim 0.9$, see Sec. 7.2) and laser background (see Sec. 2). We calculate the transmission spectrum with imperfect polarization $T_P(\omega)$ by computing a weighted average of transmission spectra:

$$T_P(\omega) = P^2 T(\omega) + P(1-P)T_1(\omega) + (1-P)PT_2(\omega) + (1-P)^2 T_0(\omega), \tag{13}$$

where $T(\omega)$, $T_1(\omega)$, $T_2(\omega)$ and $T_0(\omega)$ are all given by Eqn. 10 with $\{g_1, g_2\}$ set to $2\pi\times\{7.3, 7.3\}$, $\{7.3, 0\}$, $\{0, 7.3\}$ and $\{0, 0\}$ GHz respectively. At each field we fit Eqn. 13 to the two-spin transmission data with only the background amplitude and phase as free parameters (for an example fit, see solid black curve in **Fig. 4B**). We determine an average background amplitude and phase over all magnetic fields (data in **Fig. 4D**) and use these average values in our model. We then

use Eqn. 13 at various $\delta$ (which are determined at each magnetic field based on the linear fits shown in **Fig. 4C**) with the above cavity QED parameters, $P = 0.9$ and estimated background parameters to produce the theoretical avoided-crossing transmission spectrum shown in **Fig. 4E**.

## 7.5 Measurement of collective-state formation in an independent device

We also measure the formation of superradiant and subradiant states with a pair of SiV centers located in a different device on the same diamond chip. A transmission spectrum at $5\,\mathrm{K}$ near both SiV and cavity resonance is shown in **Fig. S9A**. From this measurement, we extract Purcell enhanced linewidths of $\{\Gamma_1(0), \Gamma_2(0)\} = 2\pi \times \{1.78, 2.43\}$ GHz. To measure the cavity mediated interaction between these SiV centers, we work at an atom-cavity detuning of $\Delta = 2\pi \times 70\,\mathrm{GHz}$. To demonstrate that we can bring spin-selective transitions from each SiV into resonance, we first measure the transmission spectrum of all transitions at a temperature of $5\,\mathrm{K}$ (**Fig. S9C**) as a magnetic field oriented roughly orthogonal to the SiV center's symmetry axis is ramped from $0\,\mathrm{kG}$ to $6.7\,\mathrm{kG}$. In this measurement, the spins are unpolarized, which allows us to see all spin-preserving transitions without a second pumping field. However, this random polarization causes us to average over the different combination of spin states (*e.g.* $P \sim 0.5$ in Eqn. 13), limiting the visibility of the cavity-mediated interaction.

As evident from the data **Fig. S9C**, there is no significant spectral diffusion for this pair of SiV centers, and we therefore choose not to implement the preselection sequence described in Sec. 7.1. Instead, to ensure proper initialization of both SiV centers into the correct charge state, we simply apply a $\sim 1\,\mu\mathrm{W}$ green pulse every $\sim 5\,\mathrm{ms}$ (*21*). At a temperature of $85\,\mathrm{mK}$, the spins can be polarized by applying pump lasers $\Omega_1$ and $\Omega_2$. By polarizing the spins individually, we measure the single SiV linewidths over long timescales under this periodic green illumination (similar to gray data in **Fig. 4B**): $\{\Gamma_1(\Delta), \Gamma_2(\Delta)\} = 2\pi \times \{0.65, 1.01\}$ GHz (**Fig. S9B**). Using the SiV linewidth data in **Fig. S9A** and **Fig. S9B**, the measured cavity linewidth (not shown) and Eqn. 12, we can extract the full cavity QED parameters: $\{g_1, g_1, \kappa, \gamma_1, \gamma_2\} = 2\pi \times \{5.7, 6.4, 85, 0.23, 0.49\}$ GHz.

**Fig. S9D** shows the spectrum of the two interacting spins at $85\,\mathrm{mK}$ (with both pump fields $\Omega_1$ and $\Omega_2$ applied), taken as a function of the magnitude of an external magnetic field oriented roughly $70^\circ$ from the SiV symmetry axis. Note that this is a slightly different orientation compared to the field used in the calibration data in (**Fig. S9C**), hence the two SiV centers tune in and out of resonance at a different magnetic field magnitude in (**Fig. S9D**). Although the avoided crossing is not as well resolved as in **Fig. 4D** of the main text due to the lower cooperativities (7 and 4) of these SiV centers, the formation of superradiant and subradiant states near the two-SiV resonance is evident from the enhanced intensity and broader linewidth of the superradiant state that remains on the positive-frequency side of the density plot in **Fig. S9D**. The theoretical spectrum (**Fig. S9E**) is calculated as in Sec. 7.4 and shows good agreement with the measured data.

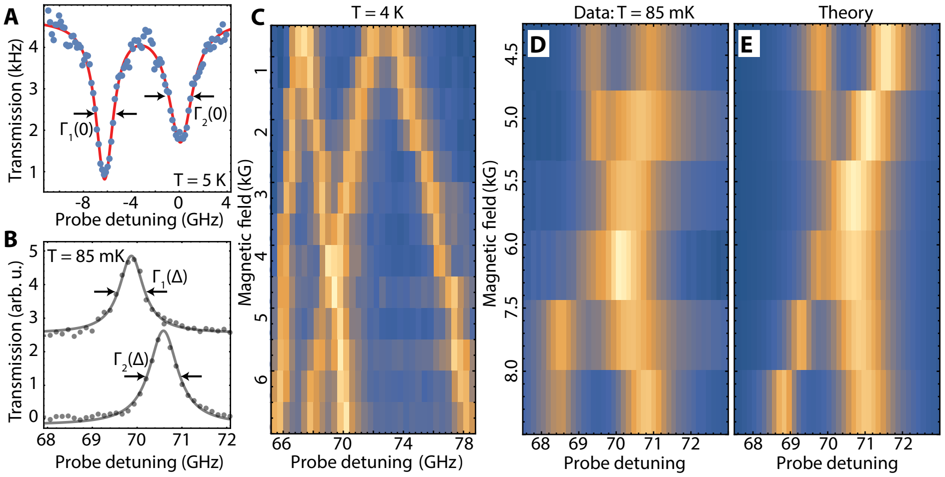


Figure S9: **SiV-SiV interaction measurement in a different device (A)** Transmission spectrum near cavity resonance ($\Delta \sim 0\,\mathrm{GHz}$). The red line shows a Bi-Lorentzian fit used to extract the Purcell-enhanced linewidths $\Gamma_1(0)$ and $\Gamma_2(0)$. **(B)** Single SiV linewidth measurements at $85\,\mathrm{mK}$ in a magnetic field oriented roughly $70^\circ$ (similar to the gray data in **Fig. 4B**). The lower data is taken at $B = 6.6\,\mathrm{kG}$ and is used to extract $\Gamma_1(\Delta)$ and the upper data (shifted vertically for clarity) is taken at $B = 8.3\,\mathrm{kG}$ and is used to extract $\Gamma_2(\Delta)$. **(C)** Zeeman calibration transmission spectrum taken as from $0\,\mathrm{kG}$ to $6.7\,\mathrm{kG}$ roughly orthogonal to the SiV symmetry axis. **(D)** Spin dependent SiV-SiV interaction at $T = 85\,\mathrm{mK}$ with both SiVs initialized into spin states that couple to the probe field taken as a function of magnetic field oriented roughly $70^\circ$ from the SiV symmetry axis. **(E)** Theoretical SiV-SiV interaction spectrum for the cavity parameters given in the text, assuming spin polarization of $90\%$ (see Sec. 7.4).

# References

42. M. Tavis, F. W. Cummings, *Physical Review* **170**, 379 (1968).

43. C. W. Gardiner, M. J. Collett, *Phys. Rev. A* **31**, 3761 (1985).

44. E. Waks, J. Vuckovic, *Phys. Rev. Lett.* **96**, 153601 (2006).
